# Supplementary material for: Static dipole polarizabilities of polyacenes using self-interaction-corrected density functional approximations
Source: arXiv:2103.05063 source file (2021-03-08)
Supplement: Supplementary file 2 [file SI.pdf]

# Supplemental information for: Static dipole polarizabilities of polyacenes using self-interaction-corrected density functional approximations

Sharmin Akter<sup>1</sup>, Yoh Yamamoto<sup>2</sup>, Rajendra R. Zope<sup>2</sup>, Tunna Baruah<sup>2</sup>

<sup>1</sup>Computational Science Program

<sup>2</sup>Department of Physics

University of Texas at El Paso, El Paso, TX, 79968

March 8, 2021

**Table S1** Cartesian coordinates for polyacenes from benzene to pentacene

---

Benzene

|    |         |         |        |
|----|---------|---------|--------|
| 12 |         |         |        |
| C  | 0.0000  | 1.3858  | 0.0000 |
| C  | 0.0000  | -1.3858 | 0.0000 |
| C  | 1.2006  | 0.6934  | 0.0000 |
| C  | -1.2006 | 0.6934  | 0.0000 |
| C  | 1.2006  | -0.6934 | 0.0000 |
| C  | -1.2006 | -0.6934 | 0.0000 |
| H  | 0.0000  | 2.4797  | 0.0000 |
| H  | 0.0000  | -2.4797 | 0.0000 |
| H  | 2.1472  | 1.2405  | 0.0000 |
| H  | -2.1472 | 1.2405  | 0.0000 |
| H  | 2.1472  | -1.2405 | 0.0000 |
| H  | -2.1472 | -1.2405 | 0.0000 |

---

## Naphthalene

|    |         |         |        |
|----|---------|---------|--------|
| 18 |         |         |        |
| C  | 1.2195  | 0.7086  | 0.0000 |
| C  | 1.2195  | -0.7086 | 0.0000 |
| C  | 0.0282  | 1.4049  | 0.0000 |
| C  | 0.0282  | -1.4049 | 0.0000 |
| C  | -1.2166 | 0.7182  | 0.0000 |
| C  | -1.2166 | -0.7182 | 0.0000 |
| C  | -3.6530 | 0.7089  | 0.0000 |
| C  | -3.6530 | -0.7089 | 0.0000 |
| C  | -2.4609 | 1.4053  | 0.0000 |
| C  | -2.4609 | -1.4053 | 0.0000 |
| H  | 0.0226  | 2.4972  | 0.0000 |
| H  | 0.0226  | -2.4972 | 0.0000 |
| H  | -2.4542 | 2.4977  | 0.0000 |
| H  | -2.4542 | -2.4977 | 0.0000 |
| H  | 2.1678  | 1.2486  | 0.0000 |
| H  | 2.1678  | -1.2486 | 0.0000 |
| H  | -4.6012 | 1.2494  | 0.0000 |
| H  | -4.6012 | -1.2494 | 0.0000 |

---

## Anthracene

|    |         |         |         |
|----|---------|---------|---------|
| 24 |         |         |         |
| C  | 1.2250  | 0.7236  | 0.0000  |
| C  | 1.2250  | -0.7236 | 0.0000  |
| C  | -0.0001 | 1.4058  | 0.0000  |
| C  | -0.0001 | -1.4058 | -0.0000 |
| C  | 3.6639  | 0.7125  | 0.0000  |
| C  | 3.6639  | -0.7125 | 0.0000  |
| C  | 2.4786  | 1.4079  | 0.0000  |
| C  | 2.4786  | -1.4079 | 0.0000  |
| C  | -1.2252 | 0.7235  | 0.0000  |
| C  | -1.2252 | -0.7235 | 0.0000  |
| C  | -3.6642 | 0.7124  | 0.0000  |
| C  | -3.6642 | -0.7124 | 0.0000  |
| C  | -2.4788 | 1.4077  | 0.0000  |
| C  | -2.4788 | -1.4077 | 0.0000  |
| H  | -0.0001 | 2.4982  | 0.0000  |
| H  | -0.0001 | -2.4982 | -0.0000 |
| H  | 2.4756  | 2.4994  | -0.0000 |
| H  | 2.4756  | -2.4994 | -0.0000 |
| H  | -2.4758 | 2.4993  | 0.0000  |
| H  | -2.4758 | -2.4993 | 0.0000  |
| H  | -4.6136 | 1.2494  | 0.0000  |
| H  | -4.6136 | -1.2494 | 0.0000  |
| H  | 4.6133  | 1.2494  | 0.0000  |
| H  | 4.6133  | -1.2494 | 0.0000  |

---

Tetracene

30

|   |         |         |         |
|---|---------|---------|---------|
| C | 1.2379  | 0.7266  | -0.0000 |
| C | 1.2379  | -0.7266 | -0.0000 |
| C | 0.0198  | 1.4085  | -0.0000 |
| C | 0.0198  | -1.4085 | -0.0000 |
| C | 3.6775  | 0.7141  | -0.0000 |
| C | 3.6775  | -0.7141 | -0.0000 |
| C | 2.4953  | 1.4097  | -0.0000 |
| C | 2.4953  | -1.4097 | -0.0000 |
| C | -1.2156 | 0.7275  | -0.0000 |
| C | -1.2156 | -0.7275 | -0.0000 |
| C | -3.6687 | 0.7266  | -0.0000 |
| C | -3.6687 | -0.7266 | -0.0000 |
| C | -2.4505 | 1.4087  | -0.0000 |
| C | -2.4505 | -1.4087 | -0.0000 |
| C | -4.9265 | 1.4092  | 0.0000  |
| C | -4.9265 | -1.4092 | 0.0000  |
| C | -6.1091 | 0.7141  | 0.0000  |
| C | -6.1091 | -0.7141 | 0.0000  |
| H | 0.0203  | 2.5012  | -0.0000 |
| H | 0.0203  | -2.5012 | -0.0000 |
| H | 2.4920  | 2.5013  | 0.0000  |
| H | 2.4920  | -2.5013 | -0.0000 |
| H | -2.4468 | 2.5013  | -0.0000 |
| H | -2.4468 | -2.5013 | -0.0000 |
| H | -4.9212 | 2.5005  | -0.0000 |
| H | -4.9212 | -2.5005 | -0.0000 |
| H | -7.0594 | 1.2496  | 0.0000  |
| H | -7.0594 | -1.2496 | 0.0000  |
| H | 4.6269  | 1.2501  | -0.0000 |
| H | 4.6269  | -1.2501 | -0.0000 |

---

---

Pentacene

|    |         |         |         |
|----|---------|---------|---------|
| 36 |         |         |         |
| C  | 1.2274  | 0.7293  | -0.0000 |
| C  | 1.2274  | -0.7293 | -0.0000 |
| C  | 0.0001  | 1.4097  | -0.0000 |
| C  | 0.0001  | -1.4097 | -0.0000 |
| C  | 3.6816  | 0.7278  | -0.0000 |
| C  | 3.6816  | -0.7279 | 0.0000  |
| C  | 2.4667  | 1.4094  | -0.0000 |
| C  | 2.4667  | -1.4094 | -0.0000 |
| C  | 4.9416  | 1.4095  | -0.0000 |
| C  | 4.9417  | -1.4095 | 0.0000  |
| C  | 6.1239  | 0.7151  | -0.0000 |
| C  | 6.1238  | -0.7151 | 0.0000  |
| C  | -1.2276 | 0.7293  | -0.0000 |
| C  | -1.2276 | -0.7293 | -0.0000 |
| C  | -3.6818 | 0.7280  | 0.0000  |
| C  | -3.6817 | -0.7280 | 0.0000  |
| C  | -2.4668 | 1.4094  | 0.0000  |
| C  | -2.4669 | -1.4094 | 0.0000  |
| C  | -4.9419 | 1.4093  | 0.0000  |
| C  | -4.9421 | -1.4093 | 0.0000  |
| C  | -6.1240 | 0.7152  | 0.0000  |
| C  | -6.1239 | -0.7152 | 0.0000  |
| H  | 0.0003  | 2.5017  | -0.0000 |
| H  | 0.0003  | -2.5017 | -0.0000 |
| H  | 2.4597  | 2.5014  | 0.0000  |
| H  | 2.4597  | -2.5014 | 0.0000  |
| H  | 4.9351  | 2.5004  | -0.0000 |
| H  | 4.9351  | -2.5004 | 0.0000  |
| H  | 7.0746  | 1.2498  | -0.0000 |
| H  | 7.0746  | -1.2498 | -0.0000 |
| H  | -2.4601 | 2.5013  | -0.0000 |
| H  | -2.4601 | -2.5013 | -0.0000 |
| H  | -4.9354 | 2.5004  | 0.0000  |
| H  | -4.9354 | -2.5004 | -0.0000 |
| H  | -7.0749 | 1.2498  | 0.0000  |
| H  | -7.0749 | -1.2498 | 0.0000  |

---
